# Supplementary material for: Learning Models from Data with Measurement Error: Tackling Underreporting
Source: arXiv:1901.09060 source file (2019-01-25)
Supplement: Supplementary file 1 [file supplementary.tex]

%%%%%%%% ICML 2019 EXAMPLE LATEX SUBMISSION FILE %%%%%%%%%%%%%%%%%

\documentclass{article}

% Recommended, but optional, packages for figures and better typesetting:
\usepackage{microtype}
\usepackage{subfigure}
\usepackage{booktabs} % for professional tables
% \usepackage{graphicx}
% \usepackage{subcaption}
% hyperref makes hyperlinks in the resulting PDF.
% If your build breaks (sometimes temporarily if a hyperlink spans a page)
% please comment out the following usepackage line and replace
% \usepackage{icml2019} with \usepackage[nohyperref]{icml2019} above.
\usepackage{hyperref}

% Attempt to make hyperref and algorithmic work together better:

% Use the following line for the initial blind version submitted for review:
\usepackage{icml2019}

% If accepted, instead use the following line for the camera-ready submission:
%\usepackage[accepted]{icml2019}

\input{includes.tex}

% The \icmltitle you define below is probably too long as a header.
% Therefore, a short form for the running title is supplied here:
\icmltitlerunning{Submission and Formatting Instructions for ICML 2019}

\begin{document}

\twocolumn[
\icmltitle{Supplementary Materials for Learning Models from Data with Measurement Error: Tackling Underreporting}

% It is OKAY to include author information, even for blind
% submissions: the style file will automatically remove it for you
% unless you've provided the [accepted] option to the icml2019
% package.

% List of affiliations: The first argument should be a (short)
% identifier you will use later to specify author affiliations
% Academic affiliations should list Department, University, City, Region, Country
% Industry affiliations should list Company, City, Region, Country

% You can specify symbols, otherwise they are numbered in order.
% Ideally, you should not use this facility. Affiliations will be numbered
% in order of appearance and this is the preferred way.
\icmlsetsymbol{equal}{*}

\begin{icmlauthorlist}
\icmlauthor{Roy Adams}{jhu}
\icmlauthor{Yuelong Ji}{jhu}
\icmlauthor{Xiaobin Wang}{jhu}
\icmlauthor{Suchi Saria}{jhu}
\end{icmlauthorlist}

\icmlaffiliation{jhu}{Johns Hopkins University, Baltimore, MD}

\icmlcorrespondingauthor{Roy Adams}{roy.james.adams@gmail.com}

% You may provide any keywords that you
% find helpful for describing your paper; these are used to populate
% the "keywords" metadata in the PDF but will not be shown in the document
\icmlkeywords{measurement error; label noise; weakly supervised learning}

\vskip 0.3in
]

% this must go after the closing bracket ] following \twocolumn[ ...

% This command actually creates the footnote in the first column
% listing the affiliations and the copyright notice.
% The command takes one argument, which is text to display at the start of the footnote.
% The \icmlEqualContribution command is standard text for equal contribution.
% Remove it (just {}) if you do not need this facility.

\printAffiliationsAndNotice{}  % leave blank if no need to mention equal contribution
% \printAffiliationsAndNotice{\icmlEqualContribution} % otherwise use the standard text.
% \sffamily
%%% Abstract %%%
% \input{abstract}

\section{Proof of Corollary 1 for probit and cloglog models}
In this section we prove Corollary 1 in Section 4.3 of the main paper for the cases of probit and cloglog regression.

\begin{proof}
Following the proof for logistic regression, a probit regression model violates the condition in Theorem 1 if

\begin{align*}
	\sqrt{2}\,\text{erf}^{-1}\left(\alpha - 1 + \alpha\,\text{erf}\left(\frac{\phi x}{\sqrt{2}}\right)\right) = \phi' x
\end{align*}

Similarly, a cloglog regression model violates the condition in Theorem 1 if 

\begin{align*}
	\log(-\log(1-\alpha+\alpha\exp(-\exp(\phi x)))) = \phi' x
\end{align*}

In both of these cases, the function on the left hand side is non-linear for $\alpha < 1$, so these equalities can only be true if $\phi x$ and $\phi' x$ are constants which is true only when $A \perp X$.
\end{proof}

\bibliography{references}
\bibliographystyle{icml2019}

%%%%%%%%%%%%%%%%%%%%%%%%%%%%%%%%%%%%%%%%%%%%%%%%%%%%%%%%%%%%%%%%%%%%%%%%%%%%%%%
%%%%%%%%%%%%%%%%%%%%%%%%%%%%%%%%%%%%%%%%%%%%%%%%%%%%%%%%%%%%%%%%%%%%%%%%%%%%%%%
% DELETE THIS PART. DO NOT PLACE CONTENT AFTER THE REFERENCES!
%%%%%%%%%%%%%%%%%%%%%%%%%%%%%%%%%%%%%%%%%%%%%%%%%%%%%%%%%%%%%%%%%%%%%%%%%%%%%%%
%%%%%%%%%%%%%%%%%%%%%%%%%%%%%%%%%%%%%%%%%%%%%%%%%%%%%%%%%%%%%%%%%%%%%%%%%%%%%%%
%%%%%%%%%%%%%%%%%%%%%%%%%%%%%%%%%%%%%%%%%%%%%%%%%%%%%%%%%%%%%%%%%%%%%%%%%%%%%%%
%%%%%%%%%%%%%%%%%%%%%%%%%%%%%%%%%%%%%%%%%%%%%%%%%%%%%%%%%%%%%%%%%%%%%%%%%%%%%%%

\end{document}
